# Supplementary material for: Highly Rectifying Conical Nanopores in Amorphous SiO2 Membranes for Nanofluidic Osmotic Power Generation and Electroosmotic Pumps
Source: arXiv:2302.01506 ancillary file (2023-05-04)
Supplement: Supplementary file 1 [file 2302_01506_SI.pdf]

## Supporting Information

### Highly Rectifying Conical Nanopores in Amorphous SiO<sub>2</sub> Membranes for Nanofluidic Osmotic Power Generation and Electroosmotic Pumps

Alexander Kiy,<sup>\*a</sup> Shankar Dutt,<sup>a</sup> Christian Notthoff,<sup>a</sup> Maria E. Toimil-Molares,<sup>b</sup> Nigel Kirby,<sup>c</sup> and Patrick Kluth<sup>a</sup>

<sup>a</sup> *Department of Materials Physics, Research School of Physics, Australian National University, Canberra ACT 2601, Australia*

<sup>b</sup> *GSI Helmholtzzentrum für Schwerionenforschung, Planckstr. 1, 64291 Darmstadt, Germany*

<sup>c</sup> *Australian Synchrotron, ANSTO, 800 Blackburn Rd Clayton VIC 3168, Australia*

\* Corresponding author: E-mail: [alexander.kiy@anu.edu.au](mailto:alexander.kiy@anu.edu.au)

#### Table of contents

|                                                  |      |
|--------------------------------------------------|------|
| 1. Hydrofluoric acid etching setup               | S-2  |
| 2. Scanning electron microscopy analysis         | S-3  |
| 2.1 Number of pores and average minimum distance | S-3  |
| 2.2 Pore base radius                             | S-4  |
| 3. Atomic force microscopy analysis              | S-5  |
| 4. Small angle X-ray scattering analysis         | S-7  |
| 5. Pore tip radius calculation                   | S-8  |
| 6. Ion transport measurements                    | S-9  |
| 7. $I - V$ data around 0 V                       | S-11 |
| References                                       | S-12 |

## 1. Hydrofluoric acid etching setup

Figure S1 shows the setup used for hydrofluoric (HF) etching of the a-SiO<sub>2</sub> membranes. The irradiated membrane is taped to a piece of wafer using Kapton tape. The membrane is then immersed into 2.5% HF that is contained in a Teflon beaker. The Kapton tape prevents HF from reaching the bottom side of the membrane and thus only the top is exposed. This enables one-sided etching of the membrane and conical nanopores are formed. After the desired etching time is reached, the membrane is removed from the HF, rinsed with deionised water and stored in deionised water until experiments are conducted.

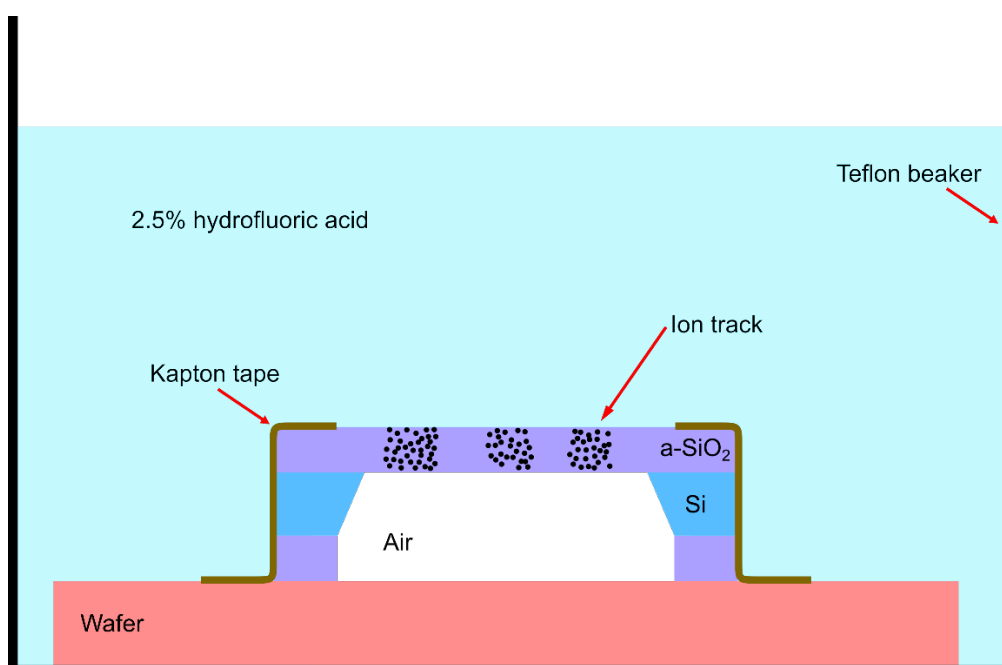

**Figure S1:** The setup used for hydrofluoric etching of the a-SiO<sub>2</sub> membranes.

## 2. Scanning electron microscopy analysis

### 2.1 Number of pores and average minimum distance

Figure S2 shows a plan-view image of the entire amorphous  $\text{SiO}_2$  (a- $\text{SiO}_2$ ) membrane obtained by scanning electron microscopy (SEM), which is the bright rectangle with an area of  $55 \times 66 \mu\text{m}^2$ . Pores can be seen on and off the membrane. Off the membrane, there is a silicon layer underneath the a- $\text{SiO}_2$  which prevents any transport through the nanopores. The pores on the membrane are numbered in red and amount to 16 in total. Note that the pores are the black dots with the white borders. The dark grey shapes are either dirt or crystallized salt. We can also determine the average minimum distance between nanopores, which is  $(7.8 \pm 4.6) \mu\text{m}$ . This is sufficient to neglect any inter-pore interactions.<sup>1</sup>

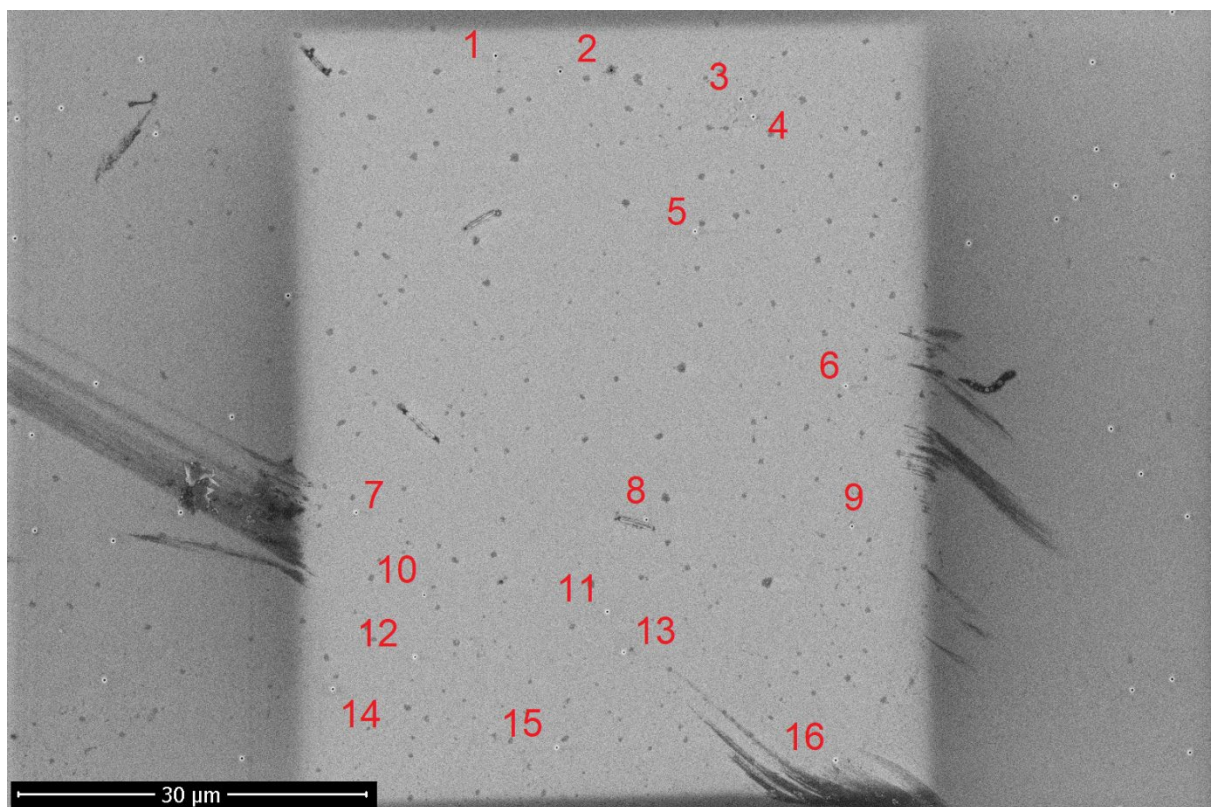

**Figure S2:** Scanning electron microscopy: Plan view of an a- $\text{SiO}_2$  membrane, which is the bright area. The nanopores on the membrane are labelled in red and amount to 16 in total.

## 2.2 Pore base radius

Figure S3(a) shows a plan view of a nanopore that was acquired using SEM. From this image, the pore base radius can be determined. Due to charging at the edge of the nanopore, which can be seen as a white ring, it is difficult to precisely determine its boundary. We have defined the edge of the pore as the edge of the charged area. An example can be seen in Figure S3(b), where the edge of the pore is highlighted in red. The base radius of this pore was determined to 166.5 nm. The average base radius of the pores was determined to  $(169 \pm 7)$  nm, where the uncertainty is the standard deviation obtained from averaging.

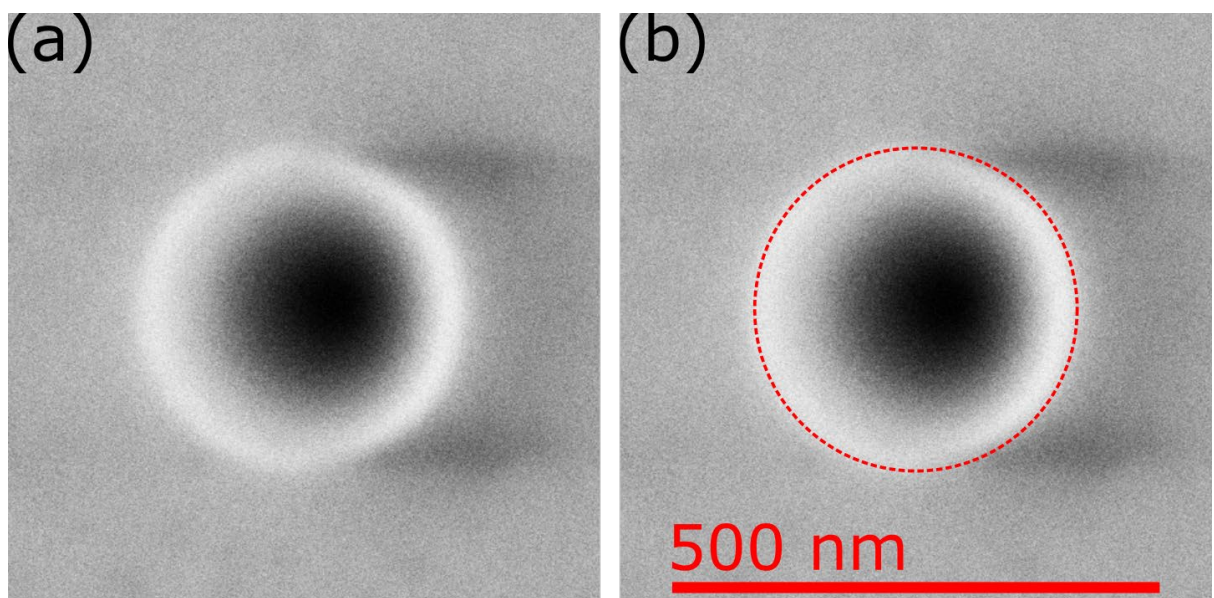

**Figure S3:** Scanning electron microscopy: (a) Plan view of a nanopore in an a-SiO<sub>2</sub> membrane. (b) The same nanopore, but the edge of the pore that was used to determine the pore base radius is highlighted in red.

### 3. Atomic force microscopy analysis

To determine the pore base radius using atomic force microscopy (AFM), three different pores were imaged in detail. For each image, the radius was measured in the x- and y-direction. An average base radius of the pores of  $(158.3 \pm 2.6)$  nm was determined. The uncertainty is the standard deviation obtained from averaging. Figure S4 shows this method for one pore. The pore does not appear perfectly circular; this is caused by the rounded AFM tip in combination with the scanning direction of the measurements process. The beginning and ending of the pore are marked with red crosses and blue crosses for the x- and y-direction, respectively. We want to note that it might look like the edge of the pore was defined too liberally. To explain this, Figure S5 shows the height profile along the y-axis. Based on that, we defined the edge of the pore where the height starts to decrease significantly. The initial curvature of the height profile is due to the curvature of the AFM tip, which has a radius of 12 nm.

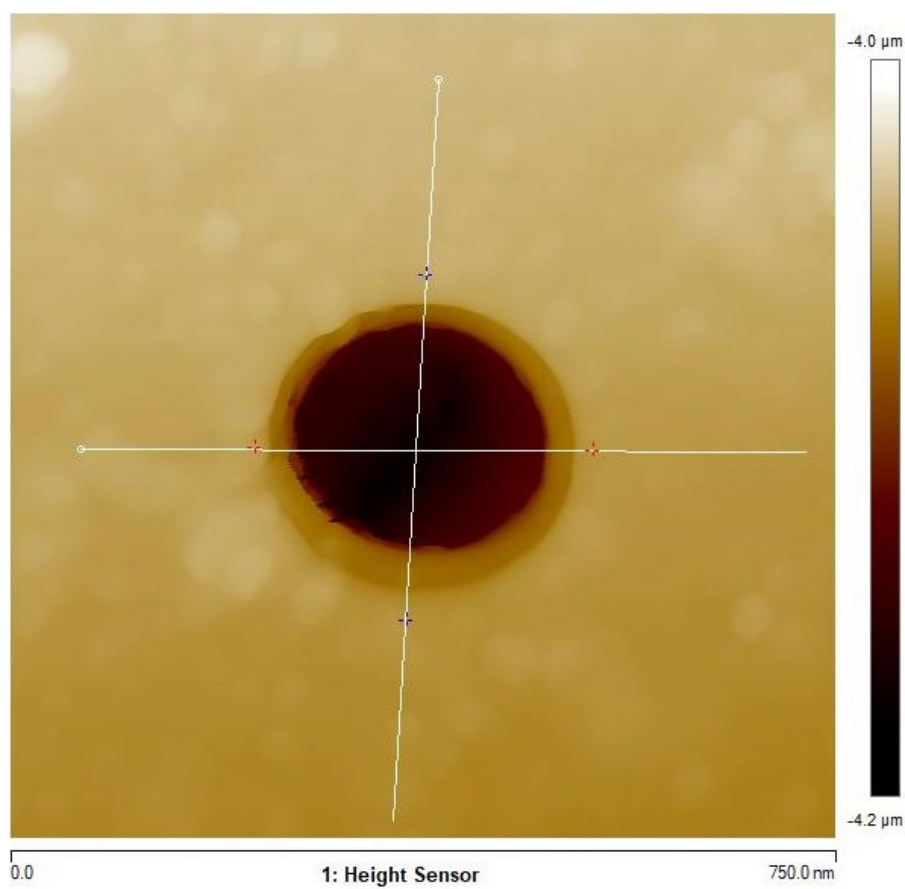

**Figure S4:** Atomic force microscopy image of a nanopore. The red and blue crosses indicate the edge of the pore in x- and y-direction, respectively.

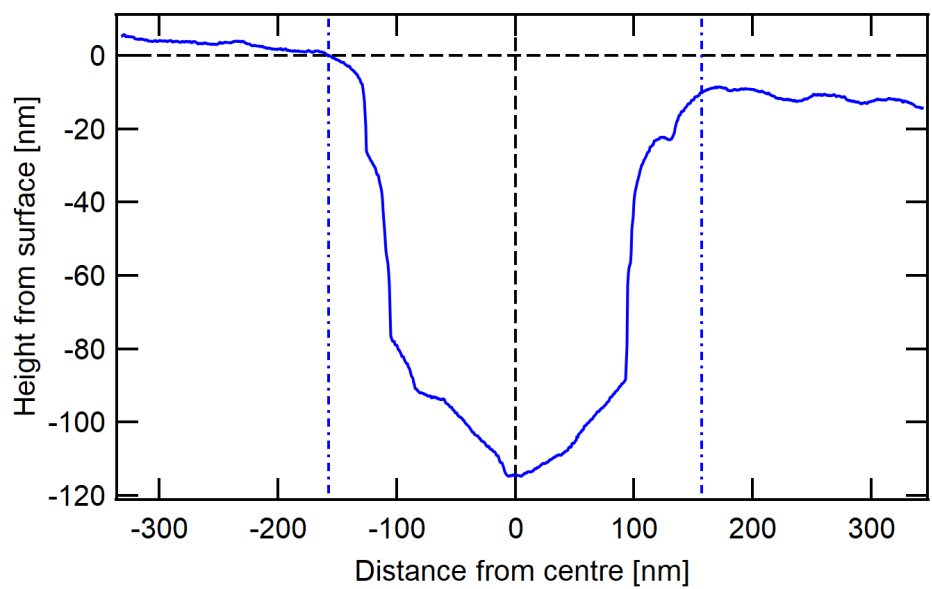

**Figure S5:** Height profile of the pore shown in Figure S4 in the y-direction. The blue vertical lines indicate the edge of the pore.

#### 4. Small angle X-ray scattering analysis

To determine the cone angle of the nanopores, synchrotron-based small angle X-ray scattering (SAXS) was performed. The membrane is tilted at angles between  $1^\circ$  to  $51^\circ$  in respect to the X-ray beam. This results in a change of the scattering pattern. By performing a fit of the 2D scattering data (Figure S6(a-e,k-o)) to our theoretical model we find that the half-cone angle of the nanopores is  $(12.6 \pm 0.1)^\circ$ . For this, all ten tilt angles are fitted simultaneously to gain a precise result. The calculated intensity is presented in Figure S6(f-j,p-t) and fits the measured data very well. A detailed explanation of the measurement and data analysis technique is given by Hadley *et al.*<sup>2</sup>

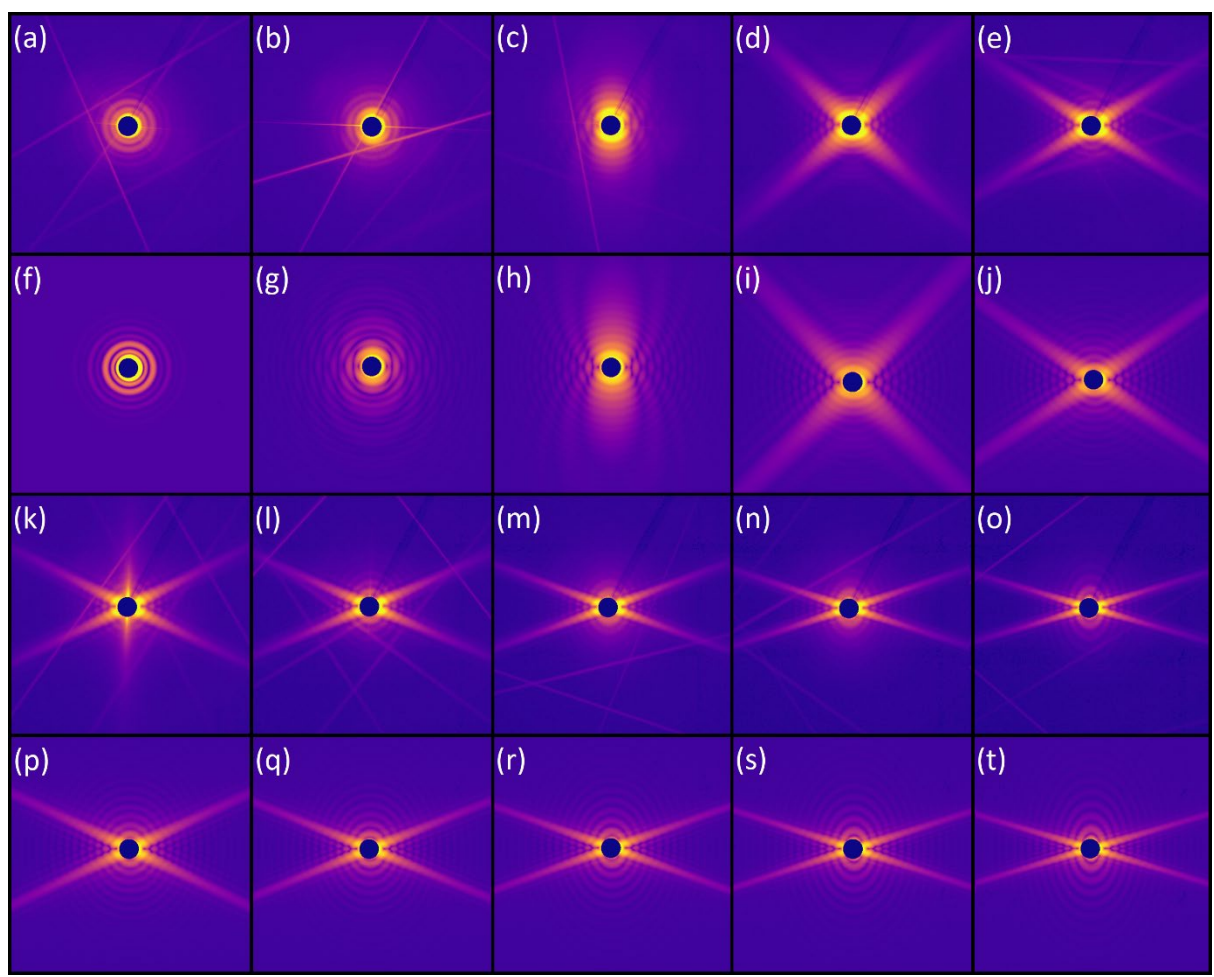

**Figure S6:** 2D scattering images (a-e,k-o) and fit to the data (f-j,p-t) of an a-SiO<sub>2</sub> nanopore membrane. (a-e) and (f-j) have tilt angles of  $1^\circ$ ,  $6^\circ$ ,  $11^\circ$ ,  $21^\circ$  and  $26^\circ$ , and (k-o) and (p-t) have tilt angles of  $31^\circ$ ,  $36^\circ$ ,  $41^\circ$ ,  $46^\circ$  and  $51^\circ$  in respect to the X-ray beam.

## 5. Pore tip radius calculation

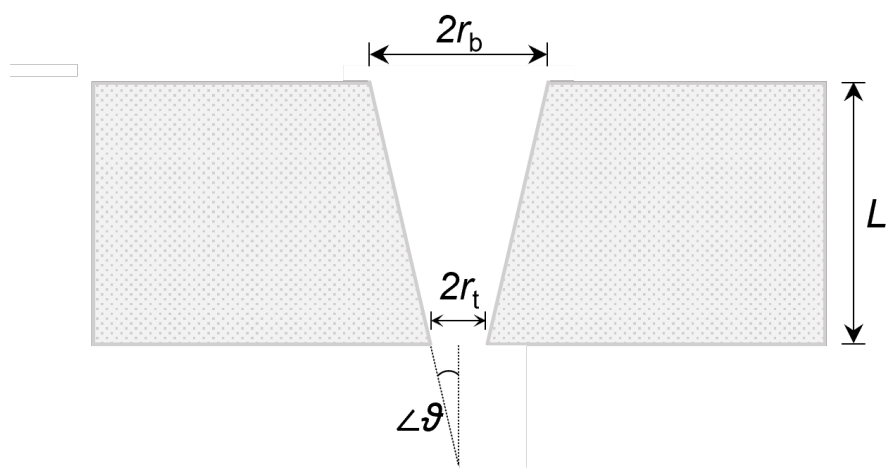

**Figure S7:** Geometry of a conical nanopore with the length  $L$ , the pore tip radius  $r_t$ , the pore base radius  $r_b$ , and the half-cone angle  $\vartheta$ .

Based on the different characterization methods used, the pore tip radius  $r_t$  can be calculated as shown in Figure S7 via the relation:

$$r_t = r_b - L \tan \vartheta$$

where the pore base radius  $r_b$  was determined using AFM and SEM. The pore length  $L$  was determined using a combination of ellipsometry and surface profiling. The half-cone angle  $\vartheta$  was determined using SAXS. The values for these three properties and the calculated pore tip radius are presented in Table S1. We calculate pore tip radii of  $(-0.3 \pm 3.1)$  and  $(11 \pm 7)$  nm for the AFM and SEM analysis, respectively. Obviously, negative pore radii are impossible, but they result by the combination of uncertainties of the different measurement techniques used. The pore base radii differ slightly, which can be attributed to the difficulty in defining the edge of the pore in either measurement technique.

**Table S1** Pore geometries determined by different measurement techniques: atomic force microscopy (AFM), scanning electron microscopy (SEM), small angle X-ray scattering (SAXS), ellipsometry and surface profiling (ell+sp).

| Pore base radius, $r_b$ [nm] | Pore length, $L$ [nm] | Half-cone angle, $\vartheta$ [°] | Pore tip radius, $r_t$ [nm] |
|------------------------------|-----------------------|----------------------------------|-----------------------------|
| AFM: $158.3 \pm 2.6$         | ell+sp: $710 \pm 5$   | SAXS: $12.6 \pm 0.1$             | $-0.3 \pm 3.1$              |
| SEM: $169 \pm 7$             | ell+sp: $710 \pm 5$   | SAXS: $12.6 \pm 0.1$             | $11 \pm 7$                  |

## 6. Ion transport measurements

All electrolyte solutions were prepared using deionised water (18.2 M $\Omega$  cm, arium® mini Sartorius ultrapure water system). Potassium chloride (KCl) was obtained from Thermo Fisher Scientific ( $\geq 99.8$  %, catalog number: AJA383-500). The pH of the solutions was adjusted using potassium hydroxide ( $\geq 85.0$  %, ChemSupply Australia, product code: PA161-500G) and hydrochloric acid (36 %, Thermo Fisher Scientific, catalogue number: R18601E). The pH and conductivity of the electrolyte were measured using an Orion Star™A215 pH/Conductivity Benchtop Multiparameter Meter from Thermo Fisher Scientific.

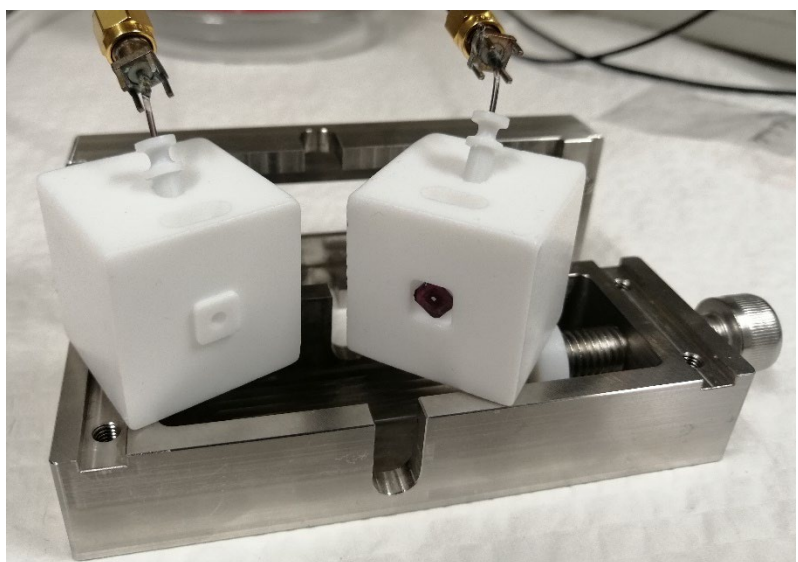

**Figure S8:** The custom-built setup used for conductometric experiments. The membrane is sealed between two fluid compartments. Using electrodes on either side of the membrane a bias voltage can be applied and the ionic current measured. The entire setup is enclosed in a stainless steel Faraday cage.

The current measurements were performed in a custom-built setup that features two Teflon cells that hold a liquid volume of 730  $\mu$ L each (see Figure S8). The nanopore membrane is sealed between two silicone gaskets and the Teflon cells, which are filled with the electrolyte. Ag/AgCl electrodes were fabricated by the reaction of silver wires ( $\varnothing 1$  mm) and sodium hypochlorite (10 %, Sigma-Aldrich) and placed in the liquid on either side of the membrane. The Teflon cells are enclosed in a stainless steel Faraday cage. The current-voltage ( $I - V$ ) curves were recorded using a Moku:Lab (Liquid Instruments) connected to a custom-built

voltage amplifier with a gain of  $10^6 \text{ V V}^{-1}$ . The voltage sweep was started at 0 V, ramped up to 1 V, reduced to -1 V and returned to 0 V with a sweep rate of  $200 \text{ mV s}^{-1}$ . This cycle was repeated until a stable current was reached, as the pore surface has to adjust to the electrolyte. Each measurement was repeated twice, and the membrane was rinsed with deionised water in between.

## 7. $I - V$ data around 0 V

Figure S9 shows a zoomed in plot of Figure 4(a) of the main text. In this Figure, the pH series is shown for 100 mM KCl for voltages between -0.1 V and 0.1 V. As the current is largely linear around 0 V, the conductance of the pores was determined in this region.

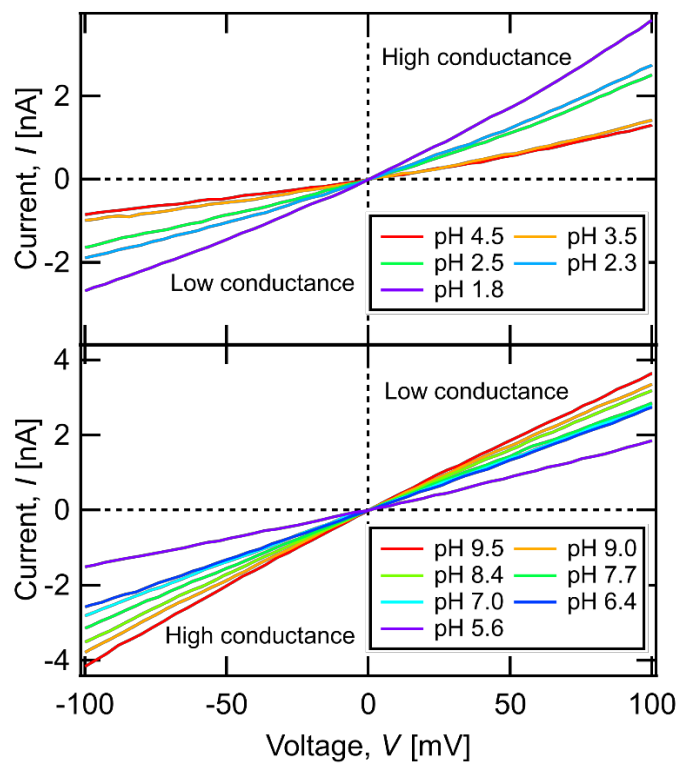

**Figure S9:**  $I - V$  curves in 100 mM KCl for the pH series in acidic and basic conditions.

## References

- (1) Cao, L.; Wen, Q.; Feng, Y.; Ji, D.; Li, H.; Li, N.; Jiang, L.; Guo, W. On the Origin of Ion Selectivity in Ultrathin Nanopores: Insights for Membrane-Scale Osmotic Energy Conversion. *Adv. Funct. Mater.* **2018**, *28*, 1804189.
- (2) Hadley, A; Notthoff, C.; Mota-Santiago, P.; Hossain, U.; Mudie, S.; Toimil-Molares, M.; Trautmann, C.; Kluth, P. Conical Etched Ion Tracks in SiO<sub>2</sub> Characterised by Small Angle X-Ray Scattering. *Nucl. Instruments Methods Phys. Res. Sect. B Beam Interact. with Mater. Atoms* **2018**, *435*, 133–136.
